# Supplementary material for: Enhancing the Authenticity of Rendered Portraits with Identity-Consistent Transfer Learning
Source: arXiv:2310.04194 source file (2023-10-06)
Supplement: Supplementary file 1 [file 6-supplementary.tex]

In this supplement, we begin with four ablation studies (Sec. \ref{sec: ablation}), followed by implementation details concerning the network architecture and dataset (Sec. \ref{sec: Implementation Details}). Next, we discuss the limitations of our work (Sec.\ref{sec: limitation}). Finally, we demonstrate our method's application in digital sample display (Sec.\ref{sec: application}) and achieve smooth results through lightweight post-processing (Sec.~\ref{sec-post-process}).

\section{Ablation Studies}
\label{sec: ablation}
In this section, we perform four ablation studies to validate the effectiveness of different components of our work.
We first evaluate the two proposed losses (Sec. \ref{sec:Ablation losses}), then our transfer-learning-based framework (Sec. \ref{sec:Ablation Framework}), the employed inversion method (Sec. \ref{sec:Ablation encode}), and finally our new high-quality rendering-style portrait dataset (Sec. \ref{sec:Ablation dataset}).

\subsection{Losses}
\label{sec:Ablation losses} We define StyleGAN2-\textit{FFHQ} generator finetuned on our \textit{DRFHQ} dataset without sketch and color constraints as the baseline. As shown in Fig.~\ref{fig:ablation}, we feed the same latent codes into various generator variants and compare the resulting portraits.

\begin{figure}[h] 
\centering
\includegraphics[width=\linewidth]{ablation.pdf}
\caption{\label{fig:ablation}
Exemplars of the ablation study of the baseline network and ours. 
From left to right, we present the images generated by StyleGAN2-\textit{FFHQ}, the baseline, the generator trained without $L_{sketch}$, the generator trained without $L_{color}$, and our full generator, respectively. 
}
% \vspace{-15pt}
\end{figure}

\textbf{Sketch loss.} 
Without the sketch constraint, the identity of the face generated by the baseline differs significantly from that of StyleGAN2-\textit{FFHQ}, thus largely affecting facial identity consistency.  %resulting in a decrease in facial identity consistency.
Thanks to $L_{color}$, the generator trained without $L_{sketch}$ generates portraits that better maintain the identity. 
However, the semantic information cannot be well preserved due to the downsampling and blurring of the images fed into the VGG16 network (see the details of the facial expressions and wrinkles in the images). 
In contrast, $L_{sketch}$ helps to keep detailed facial structure and semantics in our full model.

\textbf{Color loss.} Compared to generators trained without color constraint, those trained with color constraint can better preserve the color and lighting of the portraits generated by StyleGAN2-\textit{FFHQ}. 

\subsection{Framework}
\label{sec:Ablation Framework}
Although our sketch loss and color loss provide strong guidance for identity preservation, 
the proposed losses alone are not enough to generate satisfactory results without our carefully designed framework. 
Note that our framework includes model fine-tuning with our proposed losses, followed by inversion and generation to produce the final results. As a baseline, we directly project input rendered images into the realistic portrait latent space (StyleGAN2-\textit{FFHQ}) using our proposed losses as guidance for latent code optimization.

\begin{figure}[htbp]
\centering
\includegraphics[width=0.95\linewidth]{ablation2-0817.pdf}
\caption{\label{fig:ablation2}
Exemplars of the ablation study of the baseline method and ours. From left to right, we present the input rendered image (from the \textit{Diverse Human Faces} dataset), the result generated by the baseline method, and the result generated by ours.}
% \vspace{-15pt}
\end{figure}

As shown in Fig.~\ref{fig:ablation2}, we compare the baseline result to ours. It can be seen that the baseline produces overly smooth results, while our framework generates more realistic result.
Actually, the sketches and downsampled blurry images in the proposed losses can provide key identity information but at a coarse level, thus leading to smooth results that lack details. 
In contrast, our framework uses a $\sim$10k dataset to finetune the StyleGAN2-\textit{FFHQ} model, which is pretrained on a $\sim$70k dataset. Both large-scale datasets are rich in face features at different levels.
The fine-tuning process can effectively model the delicate details of the rendering-style faces in $G_{render}$, allowing to achieve more realistic results when transferring to $G_{real}$.

\begin{figure}[htbp]
\centering
\includegraphics[width=\linewidth]{ablation3.pdf}
\caption{\label{fig:ablation3}Exemplars of the ablation study of different inversion methods. From left to right, we present the input rendered image (from the \textit{Diverse Human Faces} dataset), the results generated using e4e, ReStyle-e4e, II2S, and ours as the inversion method.
}
% \vspace{-15pt}
\end{figure}

\subsection{Inversion}
\label{sec:Ablation encode}
In our framework, we use the latent code optimization described by Roich et al. \shortcite{10.1145/3544777} as our inversion method during inference.
We compare it to the following cutting-edge inversion approaches: e4e \cite{DBLP:journals/tog/TovANPC21}, ReStyle scheme on e4e (ReStyle-e4e) \cite{DBLP:conf/iccv/AlalufPC21}, and II2S \cite{Abdal_2019_ICCV}.

For e4e and ReStyle-e4e, we finetune their encoders pretrained on the \textit{FFHQ} dataset using our \textit{DRFHQ} dataset. Then, we input the rendered images into these finetuned encoders, respectively. 
For II2S, we use it to directly project input rendered images into $G_{rendering}$'s latent space. 
Finally, we feed these latent codes into $G_{real}$ to yield the final results for comparison. 
As shown in Fig.~\ref{fig:ablation3}, e4e changes facial identity and gender (the first row). ReStyle-e4e lacks facial details, and II2S modifies input image attributes (glasses appear in the second row of II2S). In contrast, our inversion method surpasses all others.

\subsection{Dataset}
\label{sec:Ablation dataset}

To validate the efficacy of our high-quality rendering-style portrait dataset, \textit{DRFHQ}, in enhancing facial realism, we qualitatively and quantitatively compare it with the \textit{Diverse Human Faces} dataset \cite{DHFdataset}. 
To this end, we replace our \textit{DRFHQ} dataset with \textit{Diverse Human Faces} dataset during generator fine-tuning, while maintaining method consistency.

\textbf{Qualitative comparison.} 
We enhance facial realism in rendered images using two frameworks: one based on the \textit{Diverse Human Faces} dataset and the other on our \textit{DRFHQ} datasets. Note that the input rendered portraits for inference are not part of either dataset.
As shown in Fig. \ref{fig:ablation-dataset}, our \textit{DRFHQ} dataset-based framework achieves photorealism and facial identity consistency, while the \textit{Diverse Human Faces} dataset-based framework exhibits greater disparities in geometry, color and realism. 

\begin{figure}[h]
    \centering
    \includegraphics[width=\linewidth]{fig_ablation_study_dataset.pdf}
    \caption{\label{fig:ablation-dataset} 
    Exemplars of the ablation study of the \textit{Diverse Human Faces} dataset and our \textit{DRFHQ} dataset.
    From left to right, we present the input rendered image, the results generated using the \textit{Diverse Human Faces} dataset-based framework, and ours.
    }
\end{figure}

We attribute this phenomenon to the limited diversity of the \textit{Diverse Human Faces} dataset, which consists of $\sim$7k images (after aligning and cropping) but only portrays 100 distinct identities.
In contrast, our high-quality \textit{DRFHQ} dataset contains $\sim$10k high-quality images with diverse attributes like identity, gender, age, pose, race, hairstyle, lighting, etc. This diversity effectively models the delicate rendering-style facial details during fine-tuning, leading to more realistic inference outcomes.

\textbf{Quantitative comparison.}
For quantitative evaluation, we employ LPIPS loss \cite{DBLP:conf/cvpr/ZhangIESW18} and L2 loss to assess dataset performance in information preservation. Table \ref{tab:ablation-dataset} demonstrates that our \textit{DRFHQ} dataset outperforms the \textit{Diverse Human Faces} dataset in both metrics, indicating superior overall information preservation.

\begin{table}[htbp]
\centering
\caption{Mean LPIPS and L2 losses from 150 pairs of images for the \textit{Diverse Human Faces} dataset-based and our \textit{DRFHQ} dataset-based frameworks. Lower values indicate better performance.}
\label{tab:ablation-dataset}
\begin{tabular}{ccl}
\hline
Dataset             & LPIPS↓         & L2↓            \\ \hline
DRFHQ (Ours)        & \textbf{0.135} & \textbf{0.048} \\
Diverse Human Faces & 0.176          & 0.062          \\ \hline
\end{tabular}
\end{table}

\section{Implementation Details}
\label{sec: Implementation Details}
\textbf{Networks.}
We use the StyleGAN2-ada architecture \cite{DBLP:conf/nips/KarrasAHLLA20} as the backbone for our rendering-style generator. 
StyleGAN2-\textit{FFHQ} is the official pretrained model of StyleGAN2-ada on the \textit{FFHQ} dataset.
We use the training parameters provided in the stylegan2 config of StyleGAN2-ada to finetune StyleGAN2-\textit{FFHQ} while freezing the weights of the ToRGB layers and the mapping network. We only update $G_{rendering}$ and the discriminator, while $G_{real}$ and the sketch extractor are fixed.
The training dataset is amplified with x-flips, and the fine-tuning time is about 40 minutes on 4 Tesla V100 GPUs, we stop fine-tuning when the discriminator had seen a total of 40k real images.
PyTorch \cite{pytorch2019} is utilized to train the networks and all comparisons are conducted on a desktop PC with Intel Core i7-12700F 2.10 GHz CPU, 32GB RAM and GeForce RTX 3080Ti GPU (12GB memory). All images used in the training and testing stages have a resolution of  $1024\times1024$.
{Regarding runtime performance, the average time for projecting a rendered portrait into a latent code is 27.6 seconds, with the generation of the final result only taking 0.05 seconds. All the other steps within our approach require negligible time.}

\textbf{Dataset.}
The finetuned rendering-style generator is trained using the \textit{DRFHQ} dataset's 11,399 rendering-style portraits. 
The testing images in the paper are from the \textit{Diverse Human Faces} \cite{DHFdataset} dataset and the CONNECT store \cite{CLO_connect}.

\begin{figure}[h]
    \centering
    \includegraphics[width=\linewidth]{limitation.pdf}
    \caption{\label{fig:limitations} Example of failure cases. Our method may fail in cases of faces with glasses and hats (a), complicated background (b), and large posture (c). There exist chromatic aberration and misalignment when we paste the resulting image onto the full-body apparel sample display images (d). The rendered portraits in (a, b, c) are from \textit{Diverse Human Faces} \cite{DHFdataset} dataset.
    }
\end{figure}

\section{Limitations and Future Work.} 
\label{sec: limitation}
Our method has some limitations as shown in Fig.~\ref{fig:limitations}. 
When the input faces contain accessories such as unique beards, glasses, hats, and headsets, the faces generated by our model have visible inconsistencies with the original images. This is due to the lack of corresponding relevant semantics in the \textit{FFHQ} latent space. This limitation can be addressed by enriching the diversity of photo-realistic face datasets.

Our method meets the challenges to reconstruct the background of images. We attribute this to StyleGAN's weak expressive capacity for complicated backgrounds. This limitation can be solved by removing the generated background using the alpha matte.

We notice that our approach cannot process those faces with extreme poses. This is caused by the imbalanced pose distribution in the training dataset (both \textit{FFHQ} and \textit{DRFHQ}). This can be improved by increasing the pose diversity of the dataset and retraining the StyleGAN model.

Although our method can preserve the identity of the input rendered avatar, small chromatic aberration and misalignment still exist when we paste the resulting portrait back onto the full-body apparel sample display image. To achieve seamless integration, a lightweight post-processing of the resulting portrait is further applied (see Section \ref{sec-post-process}).

\section{Application in Digital Sample Display}
\label{sec: application}
{Our proposed method can also be applied to improve the authenticity of digital sample display images.}
Fig. \ref{fig:results2} shows more exemplars where we replace the original rendering style faces with our generated realistic faces in digital apparel sample display images. Input images are courtesy of Yayat Punching at the CONNECT store \cite{CLO_connect}. 

To further validate the improvement in the authenticity of digital sample display, we collected 20 full-body apparel display images and processed them using our framework, yielding 20 pairs of images with faces of rendering-style and realistic-style, respectively.
We present these 20 pairs of test cases in sequence to 24 participants, with the original and processed images in each pair randomly displayed in position for authenticity comparison. 
Fig. \ref{fig:user-study} demonstrated that the vast majority of the full-body apparel display images {replaced faces} by our method are considered more realistic. 
This validates that stitching the resulting photo-realistic faces back onto the full-body apparel display images can effectively improve the overall authenticity.

\begin{figure}[htbp]
\centering
\pgfplotstableread[col sep=comma]{user_study_apparel_0817.csv}\datacsv
\scalebox{1}{
\begin{tikzpicture}
    \begin{axis}[
        xbar,
        y=0.42cm, enlarge y limits={true, abs value=0.75},
        xmin=0, enlarge x limits={upper, value=0.15},
        % xlabel= Number of the participants,
        % ylabel= Number of our results selected out of 40 pairs of test cases
	xmajorgrids=true,
        ytick=data,
        yticklabels from table = {\datacsv}{a},
	nodes near coords, nodes near coords align=horizontal
    ]
	\addplot table [x=b, y=a]
        {\datacsv};
    \end{axis} 
\end{tikzpicture} 
}
\caption{\label{fig:user-study}
Distribution of the user study on the authenticity of the full-body apparel display images. The $y-$axis represents the number of output images from our method selected by the participants (out of 20 pairs), and the $x-$axis represents the number of participants. Results demonstrate that stitching the resulting realistic faces back onto the full-body apparel display images can effectively improve the overall authenticity.}
\end{figure}

\section{Lightweight Post-Processing}
\label{sec-post-process}
As mentioned above, one of the applications of our method is to enhance the authenticity of digital apparel display images. However, 
as shown in Fig. \ref{fig:limitations} (d) and Fig. \ref{fig:post_process}, directly pasting the resulting  portrait back onto the original rendered digital apparel display image may lead to small chromatic aberration and misalignment.
To address this issue, we propose a lightweight post-processing method.

Specifically, we apply face parsing \cite{faceparsing} to the processed resulting portrait $x_{res}$, getting the segmentation masks of skin, brows, eyes, eyeglasses, ears, nose, mouth, lips, and hair. Then we combine them as a single mask $m$.
After that, we paste $x_{res}$ back onto the original rendered image $x$, getting $x_{res}'$,
and paste $m$ to an empty image with the same shape as $x$, getting $m'$.

To achieve smooth results, we apply erosion and Gaussian blur to $m'$, the resulting mask with smooth boundary is denoted as $\hat{m}$.
Finally, we compose the original rendered image $x$ and the intermediate image $x_{res}'$ as:
\begin{equation}
\label{equation-post-processing}
    x_{final} = \hat{m} \odot x_{res}' + (1-\hat{m}) \odot x, 
\end{equation}
where $\odot$ denotes the element-wise multiplication.

\begin{figure*}[htbp]
\centering
    \includegraphics[width=0.9\linewidth]{post_process.pdf}
    \caption{\label{fig:post_process}An overview of our lightweight post-processing method.}
\end{figure*}

\begin{figure*}[t]
\centering
   \includegraphics[width=\linewidth]{results3-2.pdf}
   \includegraphics[width=\linewidth]{apparel-display-0812.pdf}
    \caption{\label{fig:results2} 
    Our method's application in digital sample display. We replace original rendered 3D avatars' faces with photo-realistic faces generated by our method. The results show that the generated photo-real faces blend in with the rendered garments and virtual avatar bodies, effectively increasing the authenticity of the digital apparel sample display images. The input images are courtesy of Yayat Punching at the CONNECT store \cite{CLO_connect}, except for the first one in row 1.
    }
\end{figure*}
